# Supplementary material for: Reinforcement Learning on Variable Impedance Controller for High-Precision Robotic Assembly
Source: arXiv:1903.01066 source file (2019-03-20)
Supplement: Supplementary file 1 [file appendix.tex]

\section*{APPENDIX}
